# Supplementary material for: Revisiting the Resource Curse in the Age of Energy Transition: Cobalt Reserves and Conflict in Africa
Source: arXiv:2404.17713 source file (2024-04-26)
Supplement: Supplementary file 1 [file appendix_placebo.tex]

\begin{table}[htbp]\centering
\def\sym#1{\ifmmode^{#1}\else\(^{#1}\)\fi}
\caption{The Results of Placebo Treatment Year}
\resizebox{0.6\linewidth}{!}{%
\begin{tabular}{l*{3}{c}}
\hline\hline
            &\multicolumn{1}{c}{(1)}&\multicolumn{1}{c}{(2)}&\multicolumn{1}{c}{(3)}\\
            &\multicolumn{1}{c}{conflict}&\multicolumn{1}{c}{conflict}&\multicolumn{1}{c}{conflict}\\
\hline
$Cobalt \times Post_{2000}$ &      -1.260         &      -1.359         &      -1.324         \\
            &     (1.303)         &     (1.287)         &     (1.165)         \\
[1em]
Cobalt          &       2.205\sym{*}  &       2.106\sym{*}  &       1.558         \\
            &     (1.163)         &     (1.139)         &     (1.220)         \\
[1em]
$Post_{2000}$      &      -0.101         &      0.0915         &       0.368         \\
            &    (0.0951)         &     (0.188)         &     (2.208)         \\
[1em]
Controls  &          No         &          Yes         &         Yes        \\
[1em]
Country FE  &          No         &          No         &         Yes         \\
[1em]
Year FE     &          No         &          No         &         Yes         \\
\hline
\(N\)       &       39010         &       34074         &       34074         \\
\hline\hline
\multicolumn{4}{l}{\footnotesize \begin{minipage}{0.45\linewidth} \smallskip \textbf{Note:} \sym{*} \(p<0.1\), \sym{**} \(p<0.05\), \sym{***} \(p<0.01\).   \end{minipage}}\\
\end{tabular}
}
\end{table}
\label{tab: appendix_placebo}
